# Supplementary material for: Efficiently updating a covariance matrix and its LDL decomposition
Source: arXiv:2002.08831 ancillary file (2020-02-20)
Supplement: Supplementary file 1 [file 2020-march_tombs-covariance-supplementary.pdf]

Efficiently updating a covariance matrix and its LDL decomposition:

# Supplementary Material

Don March
marchdd@ornl.gov

Vandy Tombs
tombsvj@ornl.gov

February 13, 2020

## 1 Simplification for alternate form in Corollary 1.3

The alternate equation for $K$ in (3.8) follows by using Lemma 1.1 to substitute for $\overline{\mathbf{x}}_2$ and simplifying:

$$\begin{aligned}\sqrt{\frac{n+k}{n}}\left(\overline{\mathbf{y}}-\overline{\mathbf{x}}_2\right) &= \sqrt{\frac{n+k}{n}}\left(\overline{\mathbf{y}}-\frac{n\overline{\mathbf{x}}_1+k\overline{\mathbf{y}}}{n+k}\right)\\ &= \sqrt{\frac{n+k}{n}}\left(\frac{n\overline{\mathbf{y}}+k\overline{\mathbf{y}}-n\overline{\mathbf{x}}_1-k\overline{\mathbf{y}}}{n+k}\right)\\ &= \sqrt{\frac{n+k}{n}}\left(\frac{n}{n+k}\right)\left(\overline{\mathbf{y}}-\overline{\mathbf{x}}_1\right) = \sqrt{\frac{n}{n+k}}\left(\overline{\mathbf{y}}-\overline{\mathbf{x}}_1\right).\end{aligned}$$

# 2 Operation counts

## 2.1 Naive covariance matrix downdate

$$\frac{1}{n-k-1}\left(X_2-\overline{\mathbf{x}}_2\mathbf{1}_{n-k}^T\right)\left(X_2-\overline{\mathbf{x}}_2\mathbf{1}_{n-k}^T\right)^T \quad \text{where} \quad \overline{\mathbf{x}}_2=\frac{n\overline{\mathbf{x}}_1-k\overline{\mathbf{y}}}{n-k}$$

| Calculation | Description | Additions & Subtractions | Multiplications & Divisions |
|---|---|---|---|
| $\overline{\mathbf{x}}_1$ | (known) | 0 | 0 |
| $n\overline{\mathbf{x}}_1$ | scalar-vector multiplication | 0 | $m$ |
| $k\overline{\mathbf{y}}$ | vector addition | $(k-1)m$ | 0 |
| $n\overline{\mathbf{x}}_1-k\overline{\mathbf{y}}$ | vector addition | $m$ | 0 |
| $n-k$ | subtraction | 1 | 0 |
| $\overline{\mathbf{x}}_2=\frac{n\overline{\mathbf{x}}_1-k\overline{\mathbf{y}}}{n-k}$ | vector-scalar division | 0 | $m$ |
| $\overline{\mathbf{x}}_2\mathbf{1}_{n-k}^T$ | (repeat column) | 0 | 0 |
| $\left(X_2-\overline{\mathbf{x}}_2\mathbf{1}_{n-k}^T\right)$ | matrix subtraction | $(n-k)m$ | 0 |
| $\left(X_2-\overline{\mathbf{x}}_2\mathbf{1}_{n-k}^T\right)\left(X_2-\overline{\mathbf{x}}_2\mathbf{1}_{n-k}^T\right)^T$ | matrix multiplication (symmetric result) | $(n-k-1)\left(m^2+m\right)/2$ | $(n-k)\left(m^2+m\right)/2$ |
| $n-k-1$ | subtraction ($n-k$ calculated above) | 1 | 0 |
| $\frac{1}{n-k-1}\left(\left(X_2-\overline{\mathbf{x}}_2\mathbf{1}_{n-k}^T\right)\left(X_2-\overline{\mathbf{x}}_2\mathbf{1}_{n-k}^T\right)^T\right)$ | scalar-matrix multiplication | 0 | $\left(m^2+m\right)/2$ |

Total additions: $(n-k-1)\left(m^2/2\right)+(3n-k-1)(m/2)+2$

Total multiplications: $(n-k+1)\left(m^2/2\right)+(n-k+5)(m/2)$

Total operations: $(n-k)m^2+(2n-k+2)m+3$

## 2.2 Covariance matrix downdate

$$(n-k-1)\,S_2 = (n-1)\,S_1 - KK^T \quad \text{where} \quad K = Y - \left(\overline{\mathbf{y}} \pm \sqrt{\frac{n}{n-k}}\,(\overline{\mathbf{y}} - \overline{\mathbf{x}}_1)\right)\mathbf{1}_k^T$$

| Calculation | Description | Additions & Subtractions | Multiplications & Divisions |
|---|---|---|---|
| $n-k, n-k-1, n-1$ | subtraction | 3 | 0 |
| $\overline{\mathbf{x}}_1$ | (known) | 0 | 0 |
| $\overline{\mathbf{y}}$ | vector mean | $(k-1)m$ | $m$ |
| $\overline{\mathbf{y}} - \overline{\mathbf{x}}_1$ | vector subtraction | $m$ | 0 |
| $\sqrt{\frac{n}{n-k}}$ | division (+1 sqrt) | 0 | 1 |
| $\sqrt{\frac{n}{n-k}}\,(\overline{\mathbf{y}} - \overline{\mathbf{x}}_1)$ | scalar-vector multiplication | 0 | $m$ |
| $\overline{\mathbf{y}} \pm \sqrt{\frac{n}{n-k}}\,(\overline{\mathbf{y}} - \overline{\mathbf{x}}_1)$ | vector addition | $m$ | 0 |
| $\left(\overline{\mathbf{y}} \pm \sqrt{\frac{n}{n-k}}\,(\overline{\mathbf{y}} - \overline{\mathbf{x}}_1)\right)\mathbf{1}_k^T$ | (repeat column) | 0 | 0 |
| $K = Y - \left(\overline{\mathbf{y}} \pm \sqrt{\frac{n}{n-k}}\,(\overline{\mathbf{y}} - \overline{\mathbf{x}}_1)\right)\mathbf{1}_k^T$ | matrix subtraction | $km$ | 0 |
| $KK^T$ | matrix multiplication (symmetric result) | $(k-1)\,(m^2+m)/2$ | $k\,(m^2+m)/2$ |
| $(n-1)\,S_1$ | scalar-matrix multiplication ($S_1$ is also symmetric) | 0 | $(m^2+m)/2$ |
| $(n-1)\,S_1 - KK^T$ | matrix subtraction | $(m^2+m)/2$ | 0 |
| $S_2 = \frac{1}{n-k-1}\left((n-1)\,S_1 - KK^T\right)$ | scalar-matrix multiplication | 0 | $(m^2+m)/2$ |

Total additions: $(km^2 + (5k+2)m + 6)/2$

Total multiplications: $((k+2)m^2 + (k+6)m + 2)/2$

Total operations: $(k+1)m^2 + (3k+4)m + 4$, plus a square root

## 2.3 Covariance matrix LDL factorization update or downdate

Algorithm 1.

| **Calculation** | **Notes** | **Additions & Subtractions** | **Multiplications & Divisions** |
|---|---|---|---|
| $D = (n-1)D$ | | 1 | $m$ |
| $c = \sqrt{\frac{n}{n+\phi k}}$ | (+1 sqrt) | 1 | 1 |
| $\overline{\mathbf{y}}$ | vector mean | $(k-1)m$ | $m$ |
| $\boldsymbol{z} = \overline{\mathbf{y}} - c(\overline{\mathbf{y}} - \overline{\mathbf{x}}_1)$ | | $2m$ | $m$ |
| **for** $j = 1$ to $k$ | | | |
|   **for** $i = 1$ to $m$ | $km$ iterations | | |
|     $y_{ij} = y_{ij} + z_i$ | | $km$ | 0 |
|   **endfor** | | | |
|   **for** $i = 1$ to $m$ | $km$ iterations | | |
|     $\widetilde{d} = d_{ii}$ | | | |
|     $\gamma = y_{ij}/(\alpha d_{ii} + y_{ij}^2)$ | | $km$ | $3km$ |
|     $d_{ii} = d_{ii} + y_{ij}^2/\alpha$ | $y_{ij}^2$ calculated on previous line | $km$ | $km$ |
|     $\alpha = \alpha + y_{ij}^2/\widetilde{d}$ | | $km$ | $km$ |
|     **for** $p = 1$ to $m$ | $k\,(m^2-m)/2$ iterations | | |
|       $y_{pj} = y_{pj} - y_{ij}\ell_{pi}$ | | $k\,(m^2-m)/2$ | $k\,(m^2-m)/2$ |
|       $\ell_{pi} = \ell_{pi} + \gamma y_{pj}$ | | $k\,(m^2-m)/2$ | $k\,(m^2-m)/2$ |
|     **endfor** | | | |
|   **endfor** | | | |
| $D = \frac{1}{n+\phi k-1}D$ | | 1 | m |

Total additions: $km^2 + (4k+1)m + 3$

Total multiplications: $km^2 + (4k+4)m + 1$

Total operations: $2km^2 + (8k+5)m + 4$, plus a square root
